# Supplementary material for: Identifying the Effects of a Program Offer with an Application to Head Start
Source: arXiv:1711.02048 source file (2023-08-31)
Supplement: Supplementary file 2 [file latentchoicesets_supp.pdf]

# Supplement Appendix to “Identification with Latent Choice Sets”

Vishal Kamat  
Toulouse School of Economics  
University of Toulouse Capitole  
[vishal.kamat@tse-fr.eu](mailto:vishal.kamat@tse-fr.eu)

August 8, 2019

## **Abstract**

This documents provides auxiliary results along with proofs and additional mathematical derivations for all results for the author’s paper “Identification with Latent Choice Sets.”

## S.1 Motivating Discussion for Framework

In this section, I provide motivation for the framework developed in Section 3 by illustrating what standard treatment effect tools can and cannot evaluate with respect to the effects of Head Start access in the HSIS. For the purposes of this section, I introduce alternative notation to that introduced in Section 3. Specifically, since the objective is to analyze the average “treatment” effect of Head Start access, I introduce potential outcome notation where the “treatment” of interest corresponds to the receipt of Head Start access. As we will observe below, this notation will help show, using more familiar arguments without the concept of choice sets, how standard intention-to-treat and instrumental variable estimands can evaluate only so-called local average effects of Head Start access—see, for example, [Imbens and Rubin \(2015, Chapter 23\)](#) for a textbook exposition on such notation. In addition, it will allow us to emphasize why not observing where access is received corresponds to not observing the treatment of interest and, hence, complicates the application of available tools to move beyond local effects. For simplicity, the setup and notation introduced in this section does not account for the possible heterogeneity in the availability of alternative preschool access.

For a given child, let  $C$  denote the treatment of interest corresponding to an indicator for whether the parents received Head Start access or not, let  $D$  denote an indicator for whether the child was enrolled into Head Start or not, and let  $Y$  denote the child’s test score. Let  $D_1$  and  $D_0$  respectively denote the parent’s potential indicator for whether they enroll their child into Head Start with and without Head Start access, which are related to the realized indicator of Head Start enrollment by

$$D = D_1C + D_0(1 - C) . \tag{S.1}$$

Analogously, let  $Y_1$  and  $Y_0$  respectively denote the child’s potential test scores with and without Head Start access, which are related to the realized test score by

$$Y = Y_1C + Y_0(1 - C) . \tag{S.2}$$

Furthermore, let  $Z$  denote an indicator for whether the child was assigned to the treatment group or not, and let  $C_1$  and  $C_0$  respectively denote the potential indicators for whether Head Start access was received in the treatment and control group. The potential indicators for whether access was received are related to the realized indicator by

$$C = C_1Z + C_0(1 - Z) . \tag{S.3}$$

The structure of setup and the experimental design introduce certain natural restrictions between the above described variables. I formally state these restrictions in the following assumptions:

**Assumption M1.**  $D_0 = 0$  .

**Assumption M2.**  $D_0 = D_1 \implies Y_0 = Y_1$  .

**Assumption M3.**  $(Y_0, Y_1, D_0, D_1, C_0, C_1) \perp Z$  .

**Assumption M4.**  $C_1 = 1$  .

Assumption M1 states that if the child did not receive Head Start access then the parents cannot enroll their child into Head Start. Assumption M2 states that receiving Head Start access can affect test scores only if it affects the enrollment decisions, i.e. Head Start access does not directly affect outcomes but only indirectly through affecting the enrollment decision. Assumption M3 states that assignment to either the treatment or control group was random. Assumption M4 states that if the child was assigned to the treatment group then they were provided Head Start access. Note that Assumption M1 and Assumption M2 capture logical restrictions that naturally follow from the structure of the setup, whereas Assumption M3 and Assumption M4 capture restrictions that follow from the design of the experiment.

### S.1.1 Interpreting the ITT and IV Estimands

In the above described setup, the effect of Head Start access on enrollment decisions and test scores for a given child corresponds to

$$D_1 - D_0 \text{ and } Y_1 - Y_0 ,$$

i.e. the difference in potential responses with and without Head Start access. I begin by illustrating what the standard intention-to-treat (ITT) and instrumental variable (IV) estimands can evaluate with respect to these effects. The ITT estimands on enrollment decisions and test scores is defined by

$$\text{ITT}_D = E[D|Z = 1] - E[D|Z = 0] , \tag{S.4}$$

$$\text{ITT}_Y = E[Y|Z = 1] - E[Y|Z = 0] , \tag{S.5}$$

i.e. the difference in mean responses between the treatment and control group, whereas the IV estimand is defined by

$$\text{IV} = \frac{\text{ITT}_Y}{\text{ITT}_D} , \tag{S.6}$$

i.e. the ratio of the ITT estimand on test scores to that on enrollment. Using arguments from [Imbens and Angrist \(1994\)](#) modified to the above setting, the following proposition rewrites the ITT and IV estimands in terms of the underlying potential variables of the setup. The proof of this proposition is presented in Section S.6.

**Proposition S.1.1.** Suppose that Assumptions M1-M4 hold. Then

$$\begin{aligned}
\text{ITT}_D &= E[D_1 - D_0 | C_1 = 1, C_0 = 0] \cdot \text{Prob}\{C_1 = 1, C_0 = 0\} , \\
\text{ITT}_Y &= E[Y_1 - Y_0 | C_1 = 1, C_0 = 0] \cdot \text{Prob}\{C_1 = 1, C_0 = 0\} , \\
\text{IV} &= E[Y_1 - Y_0 | D_1 = 1, C_1 = 1, C_0 = 0] .
\end{aligned}$$

The above proposition states that the ITT estimands on enrollment and test scores respectively evaluate the average effect of Head Start access on enrollment and test scores conditional on the compliers times the proportion of compliers, where compliers correspond to the subgroup of children whose parents comply with their assigned status in the control group and do not receive Head Start access from the outside the experiment. Similarly, the IV estimand evaluates the average effect of Head Start access on test scores for those who would in fact enroll when access is received but again conditional on the compliers.

In summary, the above proposition shows that the ITT and IV estimands can help evaluate the conditional average effects of Head Start access which is conditional on the specific subgroup of compliers. In some cases, this subgroup is indeed the one of interest. For example, if we wanted to learn the average effect of providing Head Start access to children through the experiment then the complier subgroup is the only one of interest as they are the only ones whose receipt of Head Start access is affected by the experiment. However, in other cases, we may instead be interested in the unconditional effect for all the children. For example, if we wanted to learn the average effect of providing Head Start access to children more generally and not only through the experiment. In such cases, the objective is then to learn about

$$E[D_1 - D_0] \text{ and } E[Y_1 - Y_0] , \quad (\text{S.7})$$

i.e. the (unconditional) average effect of Head Start access on enrollment and test scores, and

$$E[Y_1 - Y_0 | D_1 = 1] , \quad (\text{S.8})$$

i.e. the (unconditional) average effect of Head Start access on test scores for those who in fact enroll when access is received. But, unless every control parent complies with their assigned status and in turn the complier subgroup coincided with the entire population, i.e.

$$\text{Prob}\{C_1 = 1, C_0 = 0\} = 1 ,$$

the ITT and IV estimands cannot evaluate the average effects of Head Start access on enrollment and test scores unconditional of the complier subgroup. In the setting of the HSIS, it is indeed the case that some control parents do not comply with their assigned status, which is indirectly revealed by the fact that some parents enroll their child into Head Start even when assigned to the control group as noted when presenting the summary statistics in Section [S.2.1](#).

### S.1.2 Moving Beyond Local Effects

More generally, following the language of the treatment effect literature, we can observe that the ITT and IV estimands allow us to only evaluate local average treatment effects (LATE) but not average treatment effects (ATE) of providing Head Start access. In this literature, a number of tools have been developed to move beyond the LATE and evaluate the ATE—see, for example, [Mogstad and Torgovitsky \(2018, Section 6\)](#) for a recent overview of such tools. Nonetheless, due to certain observational problems that arise in the setting of the HSIS, these tools generally cannot be applied to evaluate the average effects of Head Start access in the above described setup. To be specific, when applied to the above described setup, these tools typically require the distribution of

$$(Y, D, C, Z)$$

to be observed. However, in the setting of the HSIS, this is not the case. Specifically, while the experiment collected data on the test score, the enrollment decision and the treatment assignment status, it did not collect data on the receipt of program access. As a result, while we observe the values of  $Y$ ,  $D$  and  $Z$  for every child, we do not observe the value of  $C$  for any child. In other words, we do not observe the value of the “treatment” of interest whose average effect on enrollment decisions and test scores we want to evaluate.

The objective of the framework developed in [Section 3](#) is to study what we can learn about the average effects of Head Start access in such cases. In particular, it aims to show how we can exploit only the distribution of

$$(Y, D, Z)$$

to learn about the average effects of Head Start access. The framework is based on the idea that while the receipt of Head Start access is not directly observed, the structure of the model implies partial information on where access is received. For example, in the above described model, the relation in [\(S.1\)](#) and [Assumption M1](#) imply that

$$D = 1 \implies C = 1 ,$$

i.e. the child’s enrollment in Head Start reveals that parents received access to Head Start. Similarly, the relation in [\(S.3\)](#) and [Assumption M4](#) imply that

$$Z = 1 \implies C = 1 ,$$

i.e assignment to the treatment group reveals that parents in this group received Head Start access. The framework then aims to formally show how to exploit this partial information and learn about the average effects of Head Start access.

As mentioned, note that the above described model did not account for the presence of alternative preschool access for simplicity. The model presented in the framework in [Section 3](#) shows

how to expand on the above described setup and notation, and introduce their presence to study the average effects of Head Start access based on their availability. Indeed, as noted by [Feller et al. \(2016\)](#) and [Kline and Walters \(2016\)](#) in a local analysis based on the IV estimand, it can be potentially important to account for heterogeneity in the effects of Head Start access based on the availability of alternative preschools as such preschools may provide services comparable to Head Start. Similar to Head Start access, we do not directly observe whether parents received alternative preschool access and instead only observe whether parents enrolled their child in an alternative preschool. The developed framework shows how the structure of the extended model can be similarly used to exploit this partial information and learn about the average effects of Head Start access based on the availability of alternative preschool access.

While the above described treatment effect model was useful to motivate the problem behind learning the average effects of Head Start access, note that the framework in [Section 3](#) proposes an alternative more convenient representation of the model. In particular, it begins with a distinct set of care settings and the insight that receiving access to a given preschool can be framed as receiving that preschool in the choice set of care settings from which enrollment decisions are made. By exploiting this insight, it then shows how a selection model can be used to relate where access was received to the observed treatment assignment status, enrollment decision and test score. From [Section 3.1](#), observe that in this model the relationship between the various variables such as those in [\(S.1\)-\(S.3\)](#) and the logical restrictions from the setup such as [Assumption M1](#) and [Assumption M2](#) are naturally captured through the structure of the model, and the restrictions imposed by the experimental design such as [Assumption M3](#) and [Assumption M4](#) are captured in terms of [Assumption HSIS](#). In addition, from [Section 3.2](#), observe that in this model the various parameters evaluating the average effects of Head Start access such as those in [\(S.7\)](#) and [\(S.8\)](#) are defined in terms of comparing choice sets with and without Head Start in them.

## S.2 Additional Results and Details for Empirical Analysis

In this section, I provide additional empirical results and details for the empirical analysis presented in [Section 4](#).

### S.2.1 Summary Statistics

[Table S.1](#) reports the proportion of children enrolled in each care setting by the treatment and control group as measured by the enrollment decision variable for the two age cohorts. The enrollment probabilities in Head Start in the control group reveal that at least a certain proportion of parents did not comply with their assigned status and received Head Start access outside the experiment. Similarly, the enrollment probabilities in alternative preschools in treatment and control groups also

Table S.1: Proportion in each care setting by age and experimental group.

| Care setting          | Age 3     |         | Age 4     |         |
|-----------------------|-----------|---------|-----------|---------|
|                       | Treatment | Control | Treatment | Control |
| Home care             | 8.88      | 58.32   | 9.83      | 49.16   |
| Alternative preschool | 5.58      | 26.12   | 11.41     | 38.80   |
| Head Start            | 85.55     | 15.56   | 78.76     | 12.04   |
| Sample size           | 1273      | 739     | 1017      | 598     |

Table S.2: Estimates and 95% confidence intervals for the ITT and IV estimands

| Parameter        | Age 3         |               | Age 4         |               |
|------------------|---------------|---------------|---------------|---------------|
|                  | Raw           | Discretized   | Raw           | Discretized   |
| ITT <sub>D</sub> | 0.700         | 0.700         | 0.667         | 0.667         |
|                  | [0.658,0.751] | [0.658,0.751] | [0.625,0.709] | [0.625,0.709] |
| ITT <sub>Y</sub> | 0.166         | 0.171         | 0.131         | 0.140         |
|                  | [0.092,0.232] | [0.086,0.246] | [0.054,0.220] | [0.057,0.240] |
| IV               | 0.237         | 0.244         | 0.197         | 0.209         |
|                  | [0.126,0.329] | [0.120,0.350] | [0.077,0.329] | [0.082,0.358] |

*Notes:* For each quantity, the upper panel corresponds to the estimate and the lower panel corresponds to the confidence interval. The number of bootstrap draws is set to 200 and each draw is sampled at the level of the Head Start preschool.

reveal that at least a certain proportion of parents in both groups received access to an alternative preschool.

Table S.2 reports estimates of the ITT estimands on Head Start enrollment and test scores and the IV estimand, defined in Section S.1 by (S.4)-(S.6), along with 95% confidence intervals, constructed using the percentile bootstrap, for the two age cohorts. Since these results do not require the test scores to be discrete, I also report them using the raw version of the test score. The numerical results under both versions are relatively similar. As illustrated in Section S.1.1, the ITT and IV estimands will generally only help evaluate the local average effects of Head Start access for subgroup of compliers who comply with their assigned status in the control group. For parents in this complier subgroup, the ITT and IV estimates imply that the provision of Head Start access induces them to enroll their child into Head Start and also improves their child’s test scores on average.

### S.2.2 Confidence Intervals

The overall conclusions in Section 4 were based on estimated identified sets for the parameters that use the empirical distribution of the data as a sample estimate for the population distribution. In

Table S.3: 95% Confidence intervals

| Parameter      | Age 3             |                   | Age 4             |                   |
|----------------|-------------------|-------------------|-------------------|-------------------|
|                | Specification (5) | Specification (6) | Specification (5) | Specification (6) |
| $PP_{nh n}$    | 0.835             | 0.815             | 0.748             | 0.748             |
|                | 0.931             | 0.951             | 0.922             | 0.942             |
| $ATE_{nh n}$   | 0.051             | 0.031             | 0.020             | 0.000             |
|                | 1.101             | 0.987             | 1.429             | 1.222             |
| $PP_{nah na}$  | 0.145             | 0.165             | 0.214             | 0.214             |
|                | 0.875             | 0.895             | 0.828             | 0.848             |
| $ATE_{nah na}$ | -1.292            | 0.000             | -0.980            | 0.000             |
|                | 0.526             | 0.506             | 0.448             | 0.448             |

*Notes:* For each confidence interval, the upper and lower panels correspond to the lower and upper bounds, respectively. The number of bootstrap draws is set to 200 and each draw is sampled at the level of the Head Start preschool.

this section, to account for the sampling uncertainty, I present confidence intervals that cover the unknown parameter with a pre-specified probability. I construct these confidence intervals using the bootstrap procedure developed in [Deb et al. \(2018\)](#). In [Section S.3](#), I illustrate in detail how this bootstrap procedure applies to the specific structure of the linear programming problems that characterize the identified sets.<sup>1</sup>

[Table S.3](#) reports 95% confidence intervals for the various parameters for both age cohorts under the two most informative model specifications in [Table 1](#), i.e. those that impose either Assumption [MTR](#) or Assumption [Roy](#) along with Assumption [UA](#) on the baseline model. Since the bootstrap procedure in [Deb et al. \(2018\)](#) applies to only linear parameters, I do not report confidence intervals for  $ATOP_{nh|n}$  and  $ATOP_{nah|na}$ , which as noted in [Section 3.3](#) are linear-fractional parameters.

For the parameters evaluating the effect on enrollment into Head Start, the confidence sets are only slightly wider than the corresponding estimated identified sets. Under the most informative model specification, the confidence intervals for  $PP_{nh|n}$  imply that the provision of Head Start access induces between 83.5% and 93.1% of parents to enroll their three-year-old child into Head Start when access to an alternative preschool is absent. Similarly, the confidence intervals for  $PP_{nah|na}$  reveal that it induces between 14.5% and 87.5% of parents to enroll their child into Head Start when access to an alternative preschool is present.

In contrast, for the parameters measuring the effect on test scores, the confidence intervals are considerably wider than the corresponding estimated identified sets. Nonetheless, though possibly smaller in magnitude, the confidence intervals continue to suggest towards the positive benefits of Head Start access when access to an alternative preschool is absent. In particular, under the most

<sup>1</sup>In [Section S.3](#), I also present how to test the null hypothesis that the model is correctly specified, i.e.  $\mathbf{Q} \neq \emptyset$ , using the bootstrap procedure developed in [Kitamura and Stoye \(2018\)](#).

informative model specification, the confidence intervals for  $ATE_{nh|n}$  imply that the provision of Head Start access improves test scores on average between 0.051 and 1.101 standard deviations for the age three cohort when access to an alternative preschool is absent.

### S.2.3 Sensitivity Analysis

The conclusions obtained in Section 4 were based on the estimated identified sets when additional assumptions were imposed on the baseline model. In particular, the second conclusion that Head Start access improves test scores on average in the absence of alternative preschool access followed from the identified sets for  $ATE_{nh|n}$  and  $ATOP_{nh|n}$  when either Assumption **MTR** or Assumption **Roy** was imposed on the baseline model. Recall that Assumption **MTR** and Assumption **Roy** require every child in the population to satisfy certain restrictions on how their potential test scores are related to each other and on how their parents preferences are related to their potential test scores, respectively. In this section, I illustrate how we can weaken these assumptions such that only a proportion of the population is required to satisfy their respective restrictions and in turn analyze the sensitivity of the conclusion to different values of this proportion.

To this end, suppose that the population can be divided into two groups which are identical except for the fact that only one group is required to satisfy the restrictions given by the imposed assumption. More specifically, let the distribution of the summary random variable in (11) be a mixture of two distributions, i.e.

$$Q(w) = \lambda \cdot H_1(w) + (1 - \lambda) \cdot H_0(w) \quad (\text{S.9})$$

for each  $w \in \mathcal{W}$ , where  $\lambda \in [0, 1]$  denotes the proportion of the group for which the restrictions imposed by the assumption hold and  $H_1$  and  $H_0$  denote the probability mass functions of the summary random variable for the groups for which the restrictions imposed by the assumption hold and do not hold, respectively. In turn, whenever either Assumption **MTR** or Assumption **Roy** is imposed, let  $H_1$ , instead of  $Q$ , satisfy the restrictions in either (S.44) or (S.45) and let  $H_0$  remain unrestricted. Furthermore, since the only difference between the two groups is the restrictions imposed by the assumptions which are on the distribution of potential outcomes, let  $H_1$  and  $H_0$  be identical in terms of the mass they allocate to the preferences types and choice sets, i.e.

$$\sum_{(y(n), y(a), y(h)) \in \mathcal{Y}^3} H_0(w) = \sum_{(y(n), y(a), y(h)) \in \mathcal{Y}^3} H_1(w)$$

for each  $(u, c(0), c(1)) \in \mathcal{U} \times \mathcal{C} \times \mathcal{C}$ , where recall that  $w = (y(n), y(a), y(h), u, c(0), c(1))$ . Under this setup, by estimating the identified sets for  $ATE_{nh|n}$  and  $ATOP_{nh|n}$  for various pre-specified values of  $\lambda$  smaller than one, we can then analyze the sensitivity of the second conclusion noted above to weaker versions of Assumption **MTR** and Assumption **Roy**. In addition, through such an analysis, we can determine the weakest version of these assumptions required for the conclusion to hold, i.e.

Table S.4: Estimated identified sets for different values of  $\lambda$ 

| Parameter |                      | Specification (5) |        |       |       |       | Specification (6) |        |       |       |       |
|-----------|----------------------|-------------------|--------|-------|-------|-------|-------------------|--------|-------|-------|-------|
|           |                      | $\lambda$         |        |       |       |       | $\lambda$         |        |       |       |       |
|           |                      | 0.875             | 0.9    | 0.925 | 0.95  | 1     | 0.875             | 0.9    | 0.925 | 0.95  | 1     |
| Age 3     | ATE <sub>nh n</sub>  | -0.014            | 0.019  | 0.057 | 0.095 | 0.171 | -0.014            | 0.019  | 0.057 | 0.095 | 0.171 |
|           |                      | 0.981             | 0.981  | 0.981 | 0.981 | 0.981 | 0.912             | 0.907  | 0.902 | 0.897 | 0.887 |
|           | ATOP <sub>nh n</sub> | -0.016            | 0.021  | 0.063 | 0.104 | 0.187 | -0.016            | 0.021  | 0.063 | 0.104 | 0.187 |
|           |                      | 1.076             | 1.076  | 1.076 | 1.076 | 1.076 | 1.000             | 0.996  | 0.992 | 0.988 | 0.981 |
| Age 4     | ATE <sub>nh n</sub>  | -0.071            | -0.035 | 0.007 | 0.050 | 0.140 | -0.071            | -0.035 | 0.007 | 0.050 | 0.140 |
|           |                      | 1.269             | 1.269  | 1.269 | 1.269 | 1.269 | 1.150             | 1.142  | 1.133 | 1.123 | 1.102 |
|           | ATOP <sub>nh n</sub> | -0.079            | -0.039 | 0.008 | 0.055 | 0.155 | -0.079            | -0.039 | 0.008 | 0.055 | 0.155 |
|           |                      | 1.408             | 1.408  | 1.408 | 1.408 | 1.408 | 1.275             | 1.268  | 1.260 | 1.254 | 1.241 |

*Notes:* For each estimated identified set, the upper and lower panels correspond to the lower and upper bounds, respectively.

the so-called breakdown point as analyzed, for example, by [Horowitz and Manski \(1995\)](#), [Kline and Santos \(2013\)](#) and [Masten and Poirier \(2017\)](#) in various other settings.

Table S.4 reports the results of this sensitivity analysis for  $\lambda \in \{0.875, 0.9, 0.925, 0.95, 1\}$  for the two most informative specifications in Table 1, i.e. those that impose either Assumption [MTR](#) or Assumption [Roy](#) for only  $\lambda$  proportion of the population along with Assumption [UA](#) on the baseline model. As further illustrated in Section S.4, these estimated identified sets are obtained by applying a modified version of the linear programming procedure from Proposition 3.1 to the empirical distribution of the data. The estimated identified sets suggest the conclusion that Head Start access improves tests scores on average in the absence of alternative preschool access continues to hold under mild relaxations of either Assumption [MTR](#) or Assumption [Roy](#) for both age cohorts. In particular, as long as we assume that approximately at least 92.5% of the children satisfy either of these assumptions, the estimated identified sets for both age cohorts do not contain zero and in turn imply that the provision of Head Start access positively impacts test scores on average when access to an alternative preschool is absent.

#### S.2.4 Details on Discretizing Test Scores

In this section, I outline how I obtain the discrete test score outcome of interest used in the empirical results presented in Section 4 as well as the previous sections. In addition, I assess the sensitivity of the empirical findings to alternative choices of discretizations.

The choice of discretization aimed to use the empirical distribution of the observed undiscretized test scores to ensure that the discretized test scores take values in (10). Specifically, for a pre-

specified choice of  $M$ , I take each point in (10) to be given by

$$y_m = \frac{y_m^* + y_{m-1}^*}{2}$$

such that

$$y_m^* = F^{*-1} \left( m \cdot \frac{100}{M} \right)$$

for  $m \in \mathcal{M} = \{0, \dots, M\}$ , where  $F^*$  denotes the empirical distribution of the observed undiscretized test score  $Y^*$ , i.e. each point is determined by the midpoint of two specific adjacent quantiles of the empirical distribution of the observed undiscretized test scores. Then, each observed undiscretized test score  $Y^*$  is transformed as follows to its corresponding discretized version

$$Y = \begin{cases} y_m & \text{if } Y^* \in [y_{m-1}^*, y_m^*) \text{ for } m \in \{1, \dots, M-1\} \\ y_M & \text{if } Y^* \in [y_{M-1}^*, y_M^*] \end{cases},$$

which is the version of the test score used in the analysis. For the empirical results, I used ten support points for the test scores, i.e.  $M = 10$ , which ensured that the computational problems were generally tractable.

To assess the sensitivity of the empirical findings to this choice of discretization, Table S.5 reports estimated identified sets for the various parameters for the two most informative model specifications from Table 1 under two alternative more finer choices of discretizations. In particular, using the same discretization procedure described above, I consider both fifteen and twenty support points for the test scores, i.e.  $M = 15$  and  $M = 20$ .

The lower and upper bounds of the estimated identified sets for  $PP_{nh|n}$  and  $PP_{nah|na}$  are exactly identical under each choice of discretization for a given model specification. This is due to the fact that these parameters do not use any information on outcomes and hence are invariant to the choice of the discretization. However, for the parameters that measure the effects of Head Start access on test scores, the lower and upper bounds are not numerically identical. Nonetheless, the numerical differences range in absolute value between 0.03 and 0.02, which suggest that the results are relatively similar and not very sensitive to the choice of discretization.

The only important difference worth emphasizing is when the test scores are discretized to take twenty support points,  $M = 20$ . In this case, the observed data is found to be not consistent with the model specification that imposes either Assumption MTR or Assumption Roy along with Assumption UA. More formally, this occurs due to the fact that estimated version of  $\mathbf{Q}$  in (19) is empty, i.e. there does not exist a distribution of the model that can simultaneously satisfy the restrictions imposed on it by the empirical distribution of the data and by the additional assumptions.

However, it might be the case that true version of  $\mathbf{Q}$  is non-empty and only the estimated version is empty due to sampling error. To this end, the final row of Table S.5 reports the p-values of a

Table S.5: Estimated identified sets under alternative discretizations

| Parameter                  | Age 3             |             |                   |             | Age 4             |          |                   |          |
|----------------------------|-------------------|-------------|-------------------|-------------|-------------------|----------|-------------------|----------|
|                            | Specification (5) |             | Specification (6) |             | Specification (5) |          | Specification (6) |          |
|                            | $M = 15$          | $M = 20$    | $M = 15$          | $M = 20$    | $M = 15$          | $M = 20$ | $M = 15$          | $M = 20$ |
| $PP_{nh n}$                | 0.855             | $\emptyset$ | 0.855             | $\emptyset$ | 0.788             | 0.788    | 0.788             | 0.788    |
|                            | 0.911             | $\emptyset$ | 0.911             | $\emptyset$ | 0.902             | 0.902    | 0.902             | 0.902    |
| $ATE_{nh n}$               | 0.174             | $\emptyset$ | 0.174             | $\emptyset$ | 0.144             | 0.129    | 0.144             | 0.129    |
|                            | 1.035             | $\emptyset$ | 0.934             | $\emptyset$ | 1.316             | 1.345    | 1.142             | 1.165    |
| $ATOP_{nh n}$              | 0.191             | $\emptyset$ | 0.191             | $\emptyset$ | 0.160             | 0.143    | 0.160             | 0.143    |
|                            | 1.136             | $\emptyset$ | 1.031             | $\emptyset$ | 1.460             | 1.492    | 1.282             | 1.306    |
| $PP_{nah na}$              | 0.205             | $\emptyset$ | 0.205             | $\emptyset$ | 0.274             | 0.274    | 0.274             | 0.274    |
|                            | 0.855             | $\emptyset$ | 0.855             | $\emptyset$ | 0.788             | 0.788    | 0.788             | 0.788    |
| $ATE_{nah na}$             | -1.216            | $\emptyset$ | 0.000             | $\emptyset$ | -0.877            | -0.910   | 0.000             | 0.000    |
|                            | 0.446             | $\emptyset$ | 0.446             | $\emptyset$ | 0.357             | 0.351    | 0.357             | 0.351    |
| $ATOP_{nah na}$            | -1.660            | $\emptyset$ | 0.000             | $\emptyset$ | -1.285            | -1.314   | 0.000             | 0.000    |
|                            | 1.128             | $\emptyset$ | 1.128             | $\emptyset$ | 0.871             | 0.860    | 0.871             | 0.860    |
| Specification test p-value | 1.000             | 1.000       | 1.000             | 1.000       | 0.995             | 1.000    | 1.000             | 1.000    |

*Notes:* For each estimated identified set, the upper and lower panels correspond to the lower and upper bounds, respectively. For the specification test, the number of bootstrap draws is set to 200 and each draw is sampled at the level of the Head Start preschool.

model specification test outlined in Section S.3.2. For the two model specifications that are found to be inconsistent with the observed data, I find that their corresponding test statistics are very small, a value of  $6.93 \times 10^{-5}$  for both specification (5) and (6), which suggest that the violations that cause the model to be rejected are small. The p-values then imply that these violations are also statistically small and that none of the model specifications can be statistically rejected.

### S.2.5 Data and Variable Construction

The raw data used from the Head Start Impact Study (HSIS) in this paper is restricted, but access can be acquired by submitting applications to Research Connections at

<http://www.researchconnections.org/childcare/resources/19525> .

In this section, I briefly describe how the raw data was transformed to the final analysis sample used for the empirical results in the paper, which closely followed the publicly available code used to construct the final sample in Kline and Walters (2016). I organize this description in the following steps which were taken separately for each age cohort:

**Step 1:** I merged all the various data files provided by Research Connections for the HSIS and dropped observations with missing Head Start preschool IDs, where this preschool cor-

responded to that from which the child was sampled. I then made edits to this raw sample as described below.

**Step 2:** I classified the enrollment decision into the three categories used in the paper using the focal care arrangement variable provided by the HSIS data set.

**Step 3:** All observations where any of the variables used in the analysis were missing were dropped.

**Step 4:** Test score outcomes were then standardized using the test scores in the control group of the final sample.

### S.3 Statistical Inference

The identification analysis in Section 3 characterized the identified set assuming that the population distribution of the observed data was known. The empirical results in Section 4 applied this analysis to obtain an estimate of the identified set using the empirical distribution of the HSIS sample data. Here, to be precise, the HSIS sample data is given by

$$X^{(N)} = \{X_g^{(N)} : 1 \leq g \leq G\} \quad (\text{S.10})$$

where  $N$  denotes the total sample size, and

$$X_g^{(N)} = \{X_{ig} \equiv (Y_{ig}, D_{ig}, Z_{ig}) : 1 \leq i \leq N_g\}$$

denotes the cluster of observations for all the  $i$ th sampled children from the  $g$ th sampled Head Start preschool from the experiment.

In this section, I discuss two relevant procedures that account for the sample uncertainty in the estimates. The description aims to capture a sampling framework, where: (i) the random variables  $X_{ig}$  are identically distributed and uncorrelated across sampled preschools, i.e. across the index  $g$ ; and (ii) the number of sampled preschools is “large”, i.e.  $G \rightarrow \infty$ , and the number individuals per preschool is “small”, i.e.  $n_g$  is fixed for each  $g$ . In Section S.3.1 below, I first describe how to construct confidence intervals that cover the partially identified parameter with a pre-specified probability using the bootstrap procedure developed in [Deb et al. \(2018\)](#). In Section S.3.2 below, I then describe how to conduct a statistical test for whether the imposed model is correctly specified, i.e. if there exists a distribution of the latent random variables that can simultaneously satisfy the restrictions imposed by the assumptions on the model and the distribution of the observed data, using the bootstrap procedure developed in [Kitamura and Stoye \(2018\)](#).

### S.3.1 Confidence Intervals

Confidence intervals are constructed by test inversion. More specifically, I describe a test that controls the null rejection probability at a pre-specified level  $\alpha \in (0, 1)$  for the following null hypothesis

$$H_0 : \theta(Q) \equiv \sum_{w \in \mathcal{W}} a_{\text{num}}(w) \cdot Q(w) = \theta_0 , \quad (\text{S.11})$$

i.e. the parameter of interest, which is a linear function of  $Q$  is equal to a given value. Confidence interval with  $(1 - \alpha)$  coverage can then be obtained by collecting the set of all values of  $\theta_0$  that are not rejected at level  $\alpha$ .

For the purposes of describing the test, it is more useful to write the null hypothesis in an alternative manner. The null hypothesis states that there exists a  $Q \in \mathbf{Q}$  such that  $\theta(Q) = \theta_0$ . More specifically, it means that there exists a  $Q$  that satisfies the restriction imposed on it as stated in Section 3.3, i.e.

- (i)  $0 \leq Q(w) \leq 1$  for every  $w \in \mathcal{W}$  ,
- (ii)  $\sum_{w \in \mathcal{W}} Q(w) = 1$  ,
- (iii)  $\sum_{w \in \mathcal{W}_x} Q(w) = \text{Prob}\{Y = y, D = d | Z = z\}$  for every  $x = (y, d, z) \in \mathcal{X}$  ,
- (iv)  $\sum_{w \in \mathcal{W}_s} Q(w) = 0$  for every  $s \in \mathcal{S}$  ,

such that this  $Q$  can result in the parameter being equal to  $\theta_0$ , i.e.

$$\sum_{w \in \mathcal{W}} a_{\text{num}}(w) \cdot Q(w) = \theta_0 .$$

In order to state how this null hypothesis can then be equivalently restated, I first introduce some additional notation. Denote by  $\mathcal{W}^\dagger$  the set of all  $w \in \mathcal{W}$  that is not restricted to have zero probability by restriction (iv) above, i.e.  $Q(w)$  is not imposed to be zero by some  $s \in \mathcal{S}$ . Further, for shorthand notation, denote by

$$P(x) \equiv \text{Prob}\{Y = y, D = d | Z = z\}$$

for every  $x = (y, d, z) \in \mathcal{X}$ . Using this notation, note that the restriction in (iii) above can be restated as

$$\sum_{w \in \mathcal{W}_x^\dagger} Q(w) = P(x)$$

for every  $x = (y, d, z) \in \mathcal{X}$ , where  $\mathcal{W}_x^\dagger = \mathcal{W}^\dagger \cap \mathcal{W}_x$ . Then, the null hypothesis in (S.11) can be equivalently restated as

$$H_0 : \min_{\{Q(w): w \in \mathcal{W}^\dagger\}} \sum_{x \in \mathcal{X}} \left( P(x) - \sum_{w \in \mathcal{W}_x^\dagger} Q(w) \right)^2 = 0 , \quad (\text{S.12})$$

where  $\{Q(w) : w \in \mathcal{W}^\dagger\}$  satisfy the following restrictions:

- (i)  $0 \leq Q(w) \leq 1$  for every  $w \in \mathcal{W}^\dagger$ .
- (ii)  $\sum_{w \in \mathcal{W}^\dagger} Q(w) = 1$ .
- (iii)  $\sum_{w \in \mathcal{W}^\dagger} a_{\text{num}}(w) \cdot Q(w) = \theta_0$ .

This equivalent restatement of the null hypothesis serves two purposes. First, the sample analogue of the quantity in the restated null hypothesis provides an intuitive test statistic

$$TS_N(\theta_0) = \min_{\{Q(w): w \in \mathcal{W}^\dagger\}} G \sum_{x \in \mathcal{X}} \left( \hat{P}(x) - \sum_{w \in \mathcal{W}_x^\dagger} Q(w) \right)^2$$

such that  $\{Q(w) : w \in \mathcal{W}^\dagger\}$  satisfies the above restrictions, and where  $\hat{P}(x)$  is the sample analogue of  $P(x)$  for each  $x \in \mathcal{X}$ ; and, second, the restated version shows that the null hypothesis of interest translates into the one for which [Deb et al. \(2018\)](#) have recently proposed a bootstrap procedure with several desirable theoretical properties.

For completeness, I outline the test procedure below. The procedure importantly uses a restricted or so-called tightened version of the values that  $\{Q(w) : w \in \mathcal{W}^\dagger\}$  can take over those listed above. In order to introduced this restricted set, I need to first introduce some additional notation. To this end, denote by

$$\bar{\theta} = \max_{w \in \mathcal{W}^\dagger} a_{\text{num}}(w) \quad \text{and} \quad \underline{\theta} = \min_{w \in \mathcal{W}^\dagger} a_{\text{num}}(w) .$$

Further, denote by

$$\begin{aligned} \mathcal{H} &= \left\{ w \in \mathcal{W}^\dagger \right\} , \\ \bar{\mathcal{H}} &= \left\{ w \in \mathcal{W}^\dagger : a_{\text{num}}(w) = \bar{\theta} \right\} , \\ \underline{\mathcal{H}} &= \left\{ w \in \mathcal{W}^\dagger : a_{\text{num}}(w) = \underline{\theta} \right\} , \\ \mathcal{H}_0 &= \mathcal{H} \setminus (\bar{\mathcal{H}} \cup \underline{\mathcal{H}}) . \end{aligned}$$

Let  $\tau_N$  be a tuning parameter such that  $\tau_N \rightarrow 0$  and  $G \cdot \tau_N \rightarrow \infty$  as  $G \rightarrow \infty$ . For example, following [Deb et al. \(2018\)](#), in the empirical results presented in Section [S.2.2](#), I take<sup>2</sup>

$$\tau_N = \sqrt{\frac{\log G}{G}}.$$

Using this notation, denote the tightened version by

$$\mathcal{T}_{\tau_N}(\theta_0) = \left\{ \begin{array}{l} \sum_{w \in \mathcal{W}_x^\dagger} Q(w) = \eta(x) \\ \sum_{w \in \mathcal{W}^\dagger} a_{\text{num}} \cdot Q(w) = \theta_0 \\ \{Q(w) : w \in \mathcal{W}^\dagger\} \in \mathcal{V}_{\tau_N}(\theta_0) \\ 0 \leq Q(w) \leq 1 \text{ for } w \in \mathcal{W}^\dagger \\ \sum_{w \in \mathcal{W}^\dagger} Q(w) = 1 \end{array} \right\}, \quad (\text{S.13})$$

where

$$\mathcal{V}_{\tau_N}(\theta_0) = \left\{ \begin{array}{l} Q(w) \geq \frac{\bar{\theta} - \theta_0}{\bar{\theta} - \underline{\theta}} \cdot \frac{\tau_N}{|\underline{\mathcal{H}} \cup \mathcal{H}_0|} \text{ for } w \in \underline{\mathcal{H}}, \\ \{Q(w) : w \in \mathcal{W}^\dagger\} : Q(w) \geq \frac{\theta_0 - \underline{\theta}}{\bar{\theta} - \underline{\theta}} \cdot \frac{\tau_N}{|\bar{\mathcal{H}} \cup \mathcal{H}_0|} \text{ for } w \in \bar{\mathcal{H}}, \\ Q(w) \geq \left[ 1 - \frac{\bar{\theta} - \theta_0}{\bar{\theta} - \underline{\theta}} \cdot \frac{\tau_N}{|\underline{\mathcal{H}} \cup \mathcal{H}_0|} - \frac{\theta_0 - \underline{\theta}}{\bar{\theta} - \underline{\theta}} \cdot \frac{\tau_N}{|\bar{\mathcal{H}} \cup \mathcal{H}_0|} \right] \cdot \frac{\tau_N}{|\mathcal{H}_0|} \text{ for } w \in \mathcal{H}_0 \end{array} \right\}.$$

Then, the procedure to obtain the bootstrap versions of the test statistic consists of the following steps:

- (i) Compute the  $\tau_N$ -tightened restricted estimator of the empirical distribution of the data as follows:

$$\hat{\eta}_{\tau_n} = \arg \min_{\{\eta(x)\}_{x \in \mathcal{X}} \in \mathcal{T}_{\tau_N}(\theta_0)} G \sum_{x \in \mathcal{X}} \left( \hat{P}(x) - \eta(x) \right)^2.$$

- (ii) Define the  $\tau_N$ -tightened re-centered bootstrap estimators

$$\hat{P}_{b, \tau_n}(x) = \hat{P}_b(x) - \hat{P}(x) + \hat{\eta}_{\tau_n}(x)$$

for each  $x \in \mathcal{X}$  and for  $b = 1, \dots, B$ , where  $\hat{P}_b(x)$  is the analog of  $\hat{P}(x)$  using the bootstrap sample and  $B$  is the number of bootstrap iterations. In the empirical results, bootstrap samples are obtained by randomly drawing with replacement  $G$  clusters of Head Start preschools, i.e.  $X_g^{(N)}$ , from [\(S.10\)](#).

---

<sup>2</sup>I find this choice of  $\tau_N$  can sometimes imply that  $\mathcal{T}_{\tau_N}(\theta_0)$  is empty. To this end, I take  $\tau_N$  to be the largest value smaller than this choice to ensure that this set is non-empty.

(iii) For each  $b = 1, \dots, B$ , compute the value of the bootstrap test statistic as follows

$$TS_{b,N}(\theta_0) = \min_{\{\eta(x)\}_{x \in \mathcal{X}} \in \mathcal{T}_{\tau_N}(\theta_0)} G \sum_{x \in \mathcal{X}} \left( \hat{P}_{b,\tau_n}(x) - \eta(x) \right)^2 .$$

After performing the above procedure, the critical value  $\hat{c}(1 - \alpha, \theta_0)$  is given by the  $(1 - \alpha)$ -quantile of the bootstrap distribution of the test statistics

$$L_N(t, \theta_0) = \frac{1}{B} \sum_{b=1}^B 1\{TS_{b,N}(\theta_0) \leq t\} .$$

Then, the test for a given  $\theta_0$  can be denoted by

$$\phi_N(\theta_0) = 1\{TS_N(\theta_0) > \hat{c}(1 - \alpha, \theta_0)\} .$$

Given the bootstrap test for a given  $\theta_0$ , the  $(1 - \alpha)$ -confidence interval can be computed by

$$C_N = \{\theta_0 \in \mathbf{R} : \phi_N(\theta_0) = 0\} .$$

Note that though the optimization problems for computing the identified set were linear programming problems, this is not case for the above described procedure. In particular, steps (i) and (iii) of the procedure comprise of quadratic programming problems.

### S.3.2 Specification Test

The null hypothesis for testing whether the model is correctly specified can be stated as

$$H_0 : \mathbf{Q} \neq \emptyset , \tag{S.14}$$

i.e. there exists a distribution that satisfies the restrictions imposed on it by the assumptions and the distribution of the observed data. More specifically, it means that there exists a  $Q$  that satisfies the restriction imposed on it as stated in Section 3.3, i.e.

- (i)  $0 \leq Q(w) \leq 1$  for every  $w \in \mathcal{W}$  ,
- (ii)  $\sum_{w \in \mathcal{W}} Q(w) = 1$  ,
- (iii)  $\sum_{w \in \mathcal{W}_x} Q(w) = \text{Prob}\{Y = y, D = d | Z = z\}$  for every  $x = (y, d, z) \in \mathcal{X}$  ,
- (iv)  $\sum_{w \in \mathcal{W}_s} Q(w) = 0$  for every  $s \in \mathcal{S}$  .

Note that upper bound in restriction (i), and restriction (ii) are implied by restriction (iii). Then, analogous to the restatement of the null hypothesis in the previous section, the null hypothesis in (S.14) can also be stated as follows

$$H_0 : \min_{\{Q(w): w \in \mathcal{W}^\dagger\}} \sum_{x \in \mathcal{X}} \left( P(x) - \sum_{w \in \mathcal{W}_x^\dagger} Q(w) \right)^2 = 0 ,$$

where  $\{Q(w) : w \in \mathcal{W}^\dagger\}$  satisfy  $Q(w) \geq 0$  for every  $w \in \mathcal{W}^\dagger$ . Note that this null hypothesis is exactly equivalent to that in (S.12) except for the additional constraint introduced such that a linear projection of the distribution equals a given parameter value. The test statistic for this null hypothesis can be similarly given by

$$TS_N = \min_{\{Q(w) \geq 0: w \in \mathcal{W}^\dagger\}} G \sum_{x \in \mathcal{X}} \left( \hat{P}(x) - \sum_{w \in \mathcal{W}_x^\dagger} Q(w) \right)^2 .$$

The restated version of the null hypothesis translates into the one for which Kitamura and Stoye (2018) have recently proposed a bootstrap procedure. This procedure is similar to the one in Deb et al. (2018), and, in particular, Deb et al. (2018) build on this procedure. More specifically, it follows the exact same steps as that of the procedure described in the previous section except for the fact that it uses an alternative tightened set to that in (S.13), which is given by

$$\mathcal{T}_{\tau_N} = \left\{ \{ \eta(x) \}_{x \in \mathcal{X}} : \begin{array}{l} \sum_{w \in \mathcal{W}_x^\dagger} Q(w) = \eta(x) , \\ Q(w) \geq \frac{\tau_N}{|\mathcal{W}|^\dagger} \text{ for } w \in \mathcal{W}^\dagger . \end{array} \right\} ,$$

Give this alternative tightened set, the bootstrap versions of the test statistics can be computed use the same three steps described in the previous section. Then, using the bootstrap distribution of the test statistics, the p-value for the null hypothesis in (S.14) can be computed by

$$p_{\text{value}} = \frac{1}{B} \sum_{b=1}^B 1\{TS_{N,b} \geq TS_N\} .$$

## S.4 Modified Linear Program for Sensitivity Analysis

In this section, I illustrate the modified version of the linear program from Proposition 3.1 which is used in the sensitivity analysis presented in Section S.2.3. The arguments behind this modified version are similar to those of Proposition 3.1 presented in Section 3.3 with few differences. Instead of the unknown quantity being only the probability mass function  $Q$ , there are two additional auxiliary unknown probability mass functions  $H_0$  and  $H_1$  with support similarly contained in  $\mathcal{W}$ ,

i.e.  $H_0 : \mathcal{W} \rightarrow [0, 1]$  and  $H_1 : \mathcal{W} \rightarrow [0, 1]$  such that

$$\sum_{w \in \mathcal{W}} H_0(w) = 1 \quad \text{and} \quad \sum_{w \in \mathcal{W}} H_1(w) = 1 .$$

Given these additional unknown quantities, the sensitivity analysis then also introduces several additional restrictions over them which then indirectly introduce restrictions on  $Q$  through their relationship to it. To this end, from Section S.2.3, recall the following two types of restrictions that the analysis introduces on the auxiliary probability mass function. First, it introduces restrictions on how the two auxiliary probability mass functions are related as follows

$$\sum_{(y(n), y(a), y(h)) \in \mathcal{Y}^3} H_0(w) = \sum_{(y(n), y(a), y(h)) \in \mathcal{Y}^3} H_1(w) \quad (\text{S.15})$$

for each  $(u, c(0), c(1)) \in \mathcal{U} \times \mathcal{C} \times \mathcal{C}$ , where note that  $w = (y(n), y(a), y(h), u, c(0), c(1))$ . Second, it introduces certain restrictions only on  $H_1$  when additional assumptions such as Assumption MTR and Assumption Roy are imposed on the baseline model. More specifically, let  $\mathcal{S}_1$  denote the set of restrictions imposed on the  $H_1$  such that for each restriction  $s \in \mathcal{S}_1$  satisfies

$$\sum_{w \in \mathcal{W}_s} H_1(w) = 0 , \quad (\text{S.16})$$

where  $\mathcal{W}_s$  is a known subset of  $\mathcal{W}$ . Given these restriction on the auxiliary probability mass functions, the relationship between them and  $Q$  then captures how they indirectly impose restrictions on  $Q$ . To this end, recall that the relationship between them and  $Q$  is captured through the following restrictions

$$Q(w) = \lambda \cdot H_1(w) + (1 - \lambda) \cdot H_0(w) \quad (\text{S.17})$$

for each  $w \in \mathcal{W}$ , where  $\lambda \in [0, 1]$  is the pre-specified known sensitivity parameter. To summarize, what we know about  $Q$  from these restrictions imposed through the auxiliary distributions can then be captured by the following set

$$\mathbf{Q}_{\text{aux}} = \{Q \in \mathbf{Q}_{\mathcal{W}} : Q \text{ satisfies (S.17), and } H_0, H_1 \in \mathbf{Q}_{\mathcal{W}} \text{ satisfy (S.15), and (S.16) for each } s \in \mathcal{S}_1\} , \quad (\text{S.18})$$

where recall that  $\mathbf{Q}_{\mathcal{W}}$  is the set of all probability mass functions on the sample space  $\mathcal{W}$ .

Using the notation from Section 3.3, the identified set for a pre-specified parameter  $\theta(Q)$  and for a pre-specified sensitivity parameter  $\lambda$  can then be written as follows

$$\Theta_\lambda = \{\theta_0 \in \mathbf{R} : \theta(Q) = \theta_0 \text{ for some } Q \in \mathbf{Q}_\lambda\} , \quad (\text{S.19})$$

where

$$\mathbf{Q}_\lambda = \mathbf{Q} \cap \mathbf{Q}_{\text{aux}} \quad (\text{S.20})$$

is the intersection of the set of feasible distributions determined by restrictions directly imposed on  $Q$  by the data and assumptions as described in Section 3.3 and indirectly imposed on  $Q$  through the restrictions imposed on the auxiliary distributions as described above.

Given the linear-fractional structure of the parameter and the linear structure of all the restrictions, the following proposition states the linear program that is used to compute the identified sets for the sensitivity analysis. Indeed, given this structure, the same arguments used in the proof of Proposition 3.1 can be used to formally show this result. Moreover, note that the only difference between the linear program in this proposition and that in Proposition 3.1 is the introduction of additional variables and additional linear restrictions on these variables.

**Proposition S.4.1.** Suppose that  $\mathbf{Q}_\lambda$  in (S.20) is non-empty and the parameter characterized by (12) is such that

$$\sum_{w \in \mathcal{W}_{\text{den}}} Q(w) > 0 \quad (\text{S.21})$$

holds for every  $Q \in \mathbf{Q}_\lambda$ . Then the identified set in (S.19) can be written as

$$\Theta_\lambda = [\theta_l, \theta_u] , \quad (\text{S.22})$$

where the (sharp) lower and upper bounds of this interval are solutions to the following two linear programming problems

$$\theta_l = \min_{\gamma, \{Q(w), H_0(w), H_1(w)\}_{w \in \mathcal{W}}} \tilde{\theta}(Q) \quad \text{and} \quad \theta_u = \max_{\gamma, \{Q(w), H_0(w), H_1(w)\}_{w \in \mathcal{W}}} \tilde{\theta}(Q) , \quad (\text{S.23})$$

subject to the following constraints:

- (i)  $\gamma \geq 0$  .
- (ii)  $0 \leq Q(w) \leq \gamma$  for every  $w \in \mathcal{W}$  .
- (iii)  $\sum_{w \in \mathcal{W}} Q(w) = \gamma$  .
- (iv)  $\sum_{w \in \mathcal{W}_x} Q(w) = \gamma \cdot \text{Prob}\{Y = y, D = d | Z = z\}$  for every  $x = (y, d, z) \in \mathcal{X}$  .
- (v)  $\sum_{w \in \mathcal{W}_s} Q(w) = 0$  for every  $s \in \mathcal{S}$  .
- (vi)  $\sum_{w \in \mathcal{W}_{\text{den}}} Q(w) = 1$  .
- (vii)  $0 \leq H_0(w) \leq \gamma$  for every  $w \in \mathcal{W}$  .
- (viii)  $\sum_{w \in \mathcal{W}} H_0(w) = \gamma$  .
- (ix)  $0 \leq H_1(w) \leq \gamma$  for every  $w \in \mathcal{W}$  .

- (x)  $\sum_{w \in \mathcal{W}} H_1(w) = \gamma$  .
- (xi)  $\sum_{w \in \mathcal{W}_s} H_1(w) = 0$  for every  $s \in \mathcal{S}_1$  .
- (xii)  $Q(w) = \lambda \cdot H_1(w) + (1 - \lambda) \cdot H_0(w)$  for every  $w \in \mathcal{W}$  .
- (xiii)  $\sum_{(y(n), y(a), y(h)) \in \mathcal{Y}^3} H_0(y(n), y(a), y(h), u, c(0), c(1)) = \sum_{(y(n), y(a), y(h)) \in \mathcal{Y}^3} H_1(y(n), y(a), y(h), u, c(0), c(1))$   
for every  $(u, c(0), c(1)) \in \mathcal{U} \times \mathcal{C} \times \mathcal{C}$  .

## S.5 Generalized Framework and Additional Experiments

In this section, I present the generalized version of the framework which was developed in the context of the HSIS in Section 3 and show how it applies to examples of alternative experiments. In particular, I consider the following two experiments: the Oregon Health Insurance Experiment and a microfinance experiment studied in [Angelucci et al. \(2015\)](#).

### S.5.1 Generalized Framework

The framework described below generalizes the one developed in Section 3 in two directions. First, it does not restrict attention to solely three choice alternatives but allows for any finite set of alternatives. Second, it does not restrict attention to the assumption that assignment to the treatment group guaranteed access to a given alternative but allows for other assumptions that may arise based on the experiment. Both these generalizations are specifically relevant to ensure that the experiments described in the following two sections fit into this framework.

To this end, suppose that the various alternatives that an individual can choose from take values in the following finite set

$$\mathcal{D} = \{d_1, \dots, d_{|\mathcal{D}|}\} , \quad (\text{S.24})$$

where  $|\mathcal{D}| \geq 2$  to ensure that there are a non-trivial number of alternatives. For a given individual, let the observed variables be denoted by

$$(Y, D, Z) , \quad (\text{S.25})$$

where  $Z$  denotes an indicator for whether the individual is assigned to the treatment group or not,  $D$  denotes the alternative chosen by the individual, and  $Y$  denotes the outcome of interest for the individual. Suppose that the outcome takes values in the following known discrete set

$$\mathcal{Y} = \{y_1, \dots, y_M\} .$$

The observed variables are assumed to be generated by several underlying latent variables. Similar to the description of the HSIS setup in Section 3.1, it is convenient to describe these variables and how they are related to the observed variables through various stages.

In Stage 1, the individual obtains their choice set of alternatives by receiving access to various alternatives. Without loss of generality, let  $d_1$  denote the base alternative in  $\mathcal{D}$  where access is always received. Let  $C(1)$  and  $C(0)$  respectively denote the potential choice sets under the treatment and control groups which take values in the following set

$$\mathcal{C} = \{c \subseteq \mathcal{D} : d_1 \in c\} ,$$

i.e. the set of subsets of  $\mathcal{D}$  containing  $d_1$ . Let  $C$  denote the obtained choice set which is related to the potential choice sets through the following relationship

$$C = \begin{cases} C(1) & \text{if } Z = 1 , \\ C(0) & \text{if } Z = 0 . \end{cases}$$

In Stage 2, the individual chooses their preferred alternative from their obtained choice set. Suppose that each individual has a strict preference relationship over the set of alternatives  $\mathcal{D}$ . Let  $U$  denote the individual's preference type which takes values in  $\mathcal{U}$ , i.e. the set of  $|\mathcal{D}|!$  strict preference types. The observed choice  $D$  is then related to the preference type and obtained choice set through the following relationship

$$D = \sum_{u \in \mathcal{U}, c \in \mathcal{C}} d(u, c) 1\{U = u, C = c\} , \quad (\text{S.26})$$

where  $d(u, c)$  denotes the known choice function that corresponds to what preference type  $u \in \mathcal{U}$  would choose under a non-empty set  $c \subseteq \mathcal{D}$ . Finally, in Stage 3, the individual's outcome is realized. Let  $Y(d)$  denote the individual's potential outcome had the individual chosen alternative  $d \in \mathcal{D}$ . The observed outcome  $Y$  is related to the potential outcomes through the following relationship

$$Y = \sum_{d \in \mathcal{D}} Y(d) I\{D = d\} . \quad (\text{S.27})$$

Let the above described underlying latent variables be summarized the following variable

$$W = (Y(d_1), \dots, Y(d_{|\mathcal{D}|}), U, C(0), C(1)) , \quad (\text{S.28})$$

which takes values on the following discrete sample space  $\mathcal{W} = \mathcal{Y}^{|\mathcal{D}|} \times \mathcal{U} \times \mathcal{C}^2$ . Let  $Q$  denote the probability mass function of this summary variable and let  $Q_z$  denote the probability mass function conditional on  $Z = z \in \mathcal{Z} \equiv \{0, 1\}$ .

The observed data along with the information that the treatment assignment status provides through assumptions on the model restrict the possible values that  $Q$  and  $Q_z$  can take. In particular, the observed data imposes the following restrictions on  $Q_z$ :

$$\sum_{w \in \mathcal{W}_x} Q_z(w) = \text{Prob}\{Y = y, D = d | Z = z\} \quad (\text{S.29})$$

for all  $x = (y, d, z) \in \mathcal{Y} \times \mathcal{D} \times \mathcal{Z} \equiv \mathcal{X}$ , where  $\mathcal{W}_x$  is the set of all  $w$  in  $\mathcal{W}$  such that  $c = c(1)$  if  $z = 1$  and  $c = c(0)$  if  $z = 0$ ,  $d(u, c) = d$  and  $y = y(d)$ . Moreover, the treatment assignment status is assumed to be statistically independent of the underlying variables, which can formally be stated as the following restriction on the probability mass functions:

$$Q(w) = Q_z(w) \quad (\text{S.30})$$

for all  $w \in \mathcal{W}$  and  $z \in \mathcal{Z}$ . In turn, the restriction imposed by the data on  $Q_z$  can then directly be stated as a restriction on  $Q$  as follows:

$$\sum_{w \in \mathcal{W}_x} Q(w) = \text{Prob}\{Y = y, D = d | Z = z\} \quad (\text{S.31})$$

for all  $x = (y, d, z) \in \mathcal{X}$ , where  $\mathcal{W}_x$  is defined as before. The treatment assignment status also provides some information on the potential choice sets, where this information depends on the institutional details of the experiment. Furthermore, similar to the assumptions in Section 3.4, additional information based on the setting can also be imposed on the model. In general, suppose that all this information can be captured through a finite set of restrictions  $\mathcal{S}$  on  $Q$  such that each restriction  $s \in \mathcal{S}$  satisfies

$$\sum_{w \in \mathcal{W}_s} Q(w) = 0, \quad (\text{S.32})$$

where  $\mathcal{W}_s$  is a known subset of  $\mathcal{W}$ . Given these restriction, the set of admissible probability mass functions for the underlying latent variables is given by

$$\mathbf{Q} = \{Q \in \mathbf{Q}_{\mathcal{W}} : Q \text{ satisfies (S.31) and (S.32) for each } s \in \mathcal{S}\}, \quad (\text{S.33})$$

where  $\mathbf{Q}_{\mathcal{W}}$  denotes the set of all probability mass functions on the sample space  $\mathcal{W}$ .

In the context of the above described model, suppose that we are interested in learning about a parameter  $\theta(Q)$  that can written as follows

$$\theta(Q) = \frac{\sum_{w \in \mathcal{W}} a_{\text{num}}(w) \cdot Q(w)}{\sum_{w \in \mathcal{W}_{\text{den}}} Q(w)}, \quad (\text{S.34})$$

where  $a_{\text{num}} : \mathcal{W} \rightarrow \mathbf{R}$  is known function and  $\mathcal{W}_{\text{den}}$  is a known subset of  $\mathcal{W}$ , i.e. the parameter is a fraction of linear functions of  $Q$ . As described in Section 3.3 in the setting of the HSIS, several parameters that evaluate the average effect of receiving access correspond to such functions. Given that  $\mathbf{Q}$  stated in (S.33) and  $\theta(Q)$  stated in (S.34) are respectively equivalent to (19) and (12) stated in terms of the HSIS, what we can learn about the parameter can then directly be characterized using the linear programming procedure stated in Proposition 3.1.

As noted, the framework developed in Section 3 corresponds to a special case of the above described framework applied to the setting of the HSIS. In the following two sections, I illustrate two alternative experiments that have different settings to the HSIS, but face conceptually similar noncompliance and observational problems with respect to access. For each of these experiment, I describe how their setting fits into the above described framework, which can then be applied to evaluate the average effects of program access.

### S.5.2 Oregon Health Insurance Experiment

As described in detail in [Finkelstein et al. \(2012\)](#), the Oregon Health Insurance Experiment (OHIE) was a randomized evaluation of Oregon’s Medicaid program. In particular, the program consisted of two parts: the Oregon Health Plan (OHP) Standard and the OHP Plus. The experiment was the product of a lottery in 2008 that randomly selected individuals from a waiting list to potentially gain access to Medicaid through OHP Standard. Similar to the description of the HSIS, to briefly highlight the relevant features of this experiment, I organize the description of the OHIE into three stages as follows:

**Stage 1:** The experiment randomly assigned individuals through the lottery to either a treatment group where they received access to Medicaid through OHP Standard if they satisfied the eligibility requirements at the time the lottery was conducted, or a control group where they did not receive access to Medicaid through OHP Standard. In turn, the lottery did not guarantee Medicaid access to every treated individual as some of them may not satisfy the eligibility requirements for OHP Standard. Moreover, individuals in either group could potentially receive access to Medicaid outside the lottery by being eligible for OHP Plus or to alternative non-Medicaid insurance.

**Stage 2:** The experiment collect data on the type of insurance plan in which the individual was enrolled.

**Stage 3:** The experiment collected data on a number of outcomes related to health and health care utilization.

In Stage 1 of this experiment, similar to that of the HSIS, some control individuals were able to receive Medicaid access from outside the experiment through OHP Plus. In addition, we generally do not observe where individuals receive access as data is not collected on the insurance plans for which an individual is eligible.<sup>3</sup> However, unlike the HSIS, every treated individual was not

---

<sup>3</sup>The experiment, in fact, collected data on whether treated individuals applied to enroll into OHP Standard and the outcome of their decision on whether they were considered eligible. This observed variable in turn provides additional information on whether individuals had access to Medicaid, but falls outside the scope of the developed framework. I leave the extension of the framework to accommodate for such additional information for future work.

guaranteed Medicaid access as they may potentially not satisfy the eligibility requirements. Below, I describe how these features can be accommodated into the generalized framework and in turn be used to analyze the average effects of Medicaid access.

In this experiment, the set of alternatives in (S.24) corresponds to the set of insurance plan alternatives, which can be aggregated such that

$$\mathcal{D} = \{n, a, m\} ,$$

where  $m$  denotes Medicaid program insurance,  $a$  denotes alternative non-Medicaid insurance and  $n$  denotes no insurance. Furthermore, the observed variables in (S.25) correspond to the treatment assignment status in Stage 1, the insurance plan enrolled in Stage 2, and the outcome of interest in Stage 3. Furthermore, these observed variables can be assumed to be generated by the choice and outcome equations respectively defined in (S.26) and (S.27) using the corresponding underlying variables in (S.28).

Given the assumed relationship between the observed and underlying variables, the information provided by the data can be captured by restrictions in (S.31) based on the corresponding  $Q$  in this setting. Moreover, the information that the treatment assignment status provides can also be captured through restrictions in terms of those in (S.30) and (S.32). In particular, similar to Assumption **HSIS**, the information that the treatment assignment status provides can be first stated in terms of the following assumption on the underlying variables:

**Assumption OHIE.**

$$(i) \quad (Y(n), Y(a), Y(m), U, C(0), C(1)) \perp Z .$$

$$(ii) \quad m \in C(0) \implies m \in C(1) .$$

Assumption **OHIE**(i) states that the experiment randomly assigned individuals to the treatment and control groups and in turn implies the restriction in (S.30). Assumption **OHIE**(ii) states that if an individual receives Medicaid access in the control then that individual receives it in the treatment group. In particular, it captures the following institutional detail. If an individual receives Medicaid access in the control group then they received it through OHP Plus. In turn, they will also receive Medicaid access in the treatment group through at least OHP Plus as the lottery does not affect the eligibility for OHP Plus. Using similar arguments to the restatement of Assumption **HSIS**(ii) in (16), it is straightforward to derive that Assumption **OHIE**(ii) can be restated as

$$\sum_{w \in \mathcal{W}_{\text{OHIE}}} Q(w) = 0 ,$$

where  $\mathcal{W}_{\text{OHIE}} = \{w \in \mathcal{W} : m \in c(0) \text{ and } m \notin c(1)\}$ , i.e. it can be restated as a restriction in terms of (S.32).

Given that the above described setting of the OHIE fits in the generalized model, we can then use the linear programming procedure to learn about various parameters that evaluate the average effects of Medicaid access as long as they can be re-written in terms of (S.34) given the corresponding  $Q$  for this setup. In particular, similar to the parameters described in Section 3.2 for the HSIS, we can compare mean enrollment and outcome responses under choice sets of

$$\{n, a, m\} \text{ versus } \{n, a\}$$

to analyze average effects of Medicaid access when access to alternative insurance is available, and

$$\{n, m\} \text{ versus } \{n\}$$

to analyze average effects of Medicaid access when access to alternative insurance is absent. Similar to derivations in Section 3.3 for the HSIS, we can show that these parameters can be re-written in terms of (S.34).

### S.5.3 Microfinance Experiment

Angelucci et al. (2015) implemented an experiment in 2009 to analyze the Crédito Mujer microloan product provided to women by Compartamos Banco. Compartamos Banco is a large microfinance program or institution in Mexico, and Crédito Mujer is its group loan product, i.e. where a group of individuals is joint responsibly for the loans of their group. As described in detail in Angelucci et al. (2015), the experiment was implemented by providing access to Crédito Mujer to randomly selected geographic areas of north-central part of Sonora, a state in Mexico. Similar to the HSIS and the OHIE, to briefly highlight the relevant features of this experiment, I organize the description into three stages:

**Stage 1:** The experiment randomly assigned a given geographic area to either a treatment group where access to Crédito Mujer was provided to individuals living in that area or a control group where it was not. While the experiment verified addresses to ensure that individuals living in control group areas did not receive access, they could potentially receive access to Crédito Mujer from a treated area if, for example, they had a viable address they could use in a treated area—see Angelucci et al. (2015, Footnote 18). Moreover, individuals living in both treated and control group areas could also potentially receive access to alternative microloan products based on their availability in their respective areas.

**Stage 2:** The experiment collected data for a number of individuals in each area on where they borrowed from.

**Stage 3:** The experiment also collected data on a number of outcomes such as, for example, those related to income, labor supply and social well being.

In Stage 1 of this experiment, similar to that of the HSIS, individuals in the treatment group were provided access to Crédito Mujer through the experiment and some individuals in the control group were able to receive access to it from outside the rules of the experiment. In addition, we generally do not directly observe where individuals receive access as data is not collected on the receipt of loan access for any individual, but can only indirectly learn something about it through their treatment assignment statuses and their participation or borrowing decisions. However, unlike the HSIS where individuals could participate in only a single care setting at a given time, individuals in this experiment could be simultaneously borrowing from multiple loan programs at the same time. Below, I describe how this feature can be accommodated into the generalized framework and in turn be used to analyze the average effects of Crédito Mujer access.

In this experiment, the set of alternatives in (S.24) corresponds to the set of loan alternatives that an individual can be borrowing from, which can be aggregated such that

$$\mathcal{D} = \{n, a, m, ma\} ,$$

where  $m$  denotes the Crédito Mujer,  $a$  denotes alternative microloan products,  $ma$  denotes both Crédito Mujer and alternative products, and  $n$  denotes no microloan product. Furthermore, the observed variables in (S.25) correspond to the treatment assignment status in Stage 1, the borrowing decision in Stage 2, and the outcome of interest in Stage 3. Furthermore, these observed variables can be assumed to be generated by the choice and outcome equations respectively defined in (S.26) and (S.27) using the corresponding underlying variables in (S.28).

Given the assumed relationship between the observed and underlying variables, the information provided by the data can be captured by restrictions in (S.31) based on the corresponding  $Q$  in this setting. Moreover, the information that the treatment assignment status provides can also be captured through restrictions in terms of those in (S.30) and (S.32). In particular, similar to Assumption HSIS, the information that the treatment assignment status provides can be first stated in terms of the following assumption on the underlying variables:

**Assumption MFE.**

- (i)  $(Y(n), Y(a), Y(m), Y(ma), U, C(0), C(1)) \perp Z$  .
- (ii)  $m \in C(1)$  .
- (iii) For  $z \in \{0, 1\}$ ,  $ma \in C(z) \iff m, a \in C(z)$  .

Assumption MFE(i) states that the experiment randomly assigned individuals to the treatment and control groups and in turn implies the restriction in (S.30). Assumption MFE(ii) states that if an individual lives in an area assigned to the treatment group then the individual receives access to Crédito Mujer. Assumption MFE(iii) states that, for both in the treatment and control group,

an individual receives access to both Crédito Mujer and alternative products if and only if the individual also has access to each product individually. Note that while Assumption **MFE**(iii) is not a feature of the treatment assignment status, it is a logical feature of the way the set of choice alternatives is defined in this setting. Using similar arguments to the restatement of Assumption **HSIS**(ii) in (16), it is straightforward to derive that Assumption **MFE**(ii) and Assumption **MFE**(iii) can respectively be restated as

$$\sum_{w \in \mathcal{W}_{\text{MFEii}}} Q(w) = 0$$

and

$$\sum_{w \in \mathcal{W}_{\text{MFEiii}}} Q(w) = 0 ,$$

where  $\mathcal{W}_{\text{MFEii}} = \{w \in \mathcal{W} : m \notin c(1)\}$  and  $\mathcal{W}_{\text{MFEiii}} = \{w \in \mathcal{W} : ma \in c(0), m, a \notin c(0)\} \cup \{w \in \mathcal{W} : m, a \in c(0), ma \notin c(0)\} \cup \{w \in \mathcal{W} : ma \in c(1), m, a \notin c(1)\} \cup \{w \in \mathcal{W} : m, a \in c(1), ma \notin c(1)\}$ , i.e. both of the assumptions can be restated as restrictions in terms of (S.32).

Given that the above described setting of the experiment fits in the generalized model, we can then use the linear programming procedure to learn about various parameters that evaluate the average effects of Crédito Mujer access as long as they can be re-written in terms of (S.34) given the corresponding  $Q$  for this setup. In particular, similar to the parameters described in Section 3.2 for the HSIS, we can compare mean borrowing decisions and outcome responses under choice sets of

$$\{n, a, m, ma\} \text{ versus } \{n, a\}$$

to analyze average effects of Crédito Mujer access when access to alternative microloan products is available, and

$$\{n, m\} \text{ versus } \{n\}$$

to analyze average effects of Crédito Mujer access when access to alternative microloan products is absent. Similar to derivations in Section 3.3 for the HSIS, we can show that these parameters can be re-written in terms of (S.34).

## S.6 Proof of Propositions and Additional Derivations

### S.6.1 Proof of Proposition 3.1

To begin, note that  $\mathbf{Q}_{\mathcal{W}}$  is closed and convex. Further, note that  $\mathbf{Q}$  is a set of distributions in  $\mathbf{Q}_{\mathcal{W}}$  that is obtained by placing linear constraints imposed by the data in (15) and by assumptions in (17) for each  $s \in \mathcal{S}$ . This in turn implies that  $\mathbf{Q}$  is a closed and convex set as well.

Next, it follows from (12) that  $\theta(Q)$  is a linear-fractional function of  $Q$  where the denominator is required to be positive, i.e. (20) holds, for every  $Q \in \mathbf{Q}$ . Along with  $\mathbf{Q}$  being a closed and convex set, this in turn implies that  $\theta(\mathbf{Q})$  is a closed and convex set in  $\mathbf{R}$ . More specifically, it follows that the identified set in (18) can be written as the closed interval in (21), where the lower bound and upper bound are given by

$$\theta_l = \min_{Q \in \mathbf{Q}} \theta(Q) \quad \text{and} \quad \theta_u = \max_{Q \in \mathbf{Q}} \theta(Q) . \quad (\text{S.35})$$

In order to complete the proof, note that the optimization problems in (S.35) have linear-fractional objectives due to the structure of the parameter in (12) and a finite number of linear constraints as guaranteed by the data restrictions in (15) and the structure of the imposed restrictions in (17) for each  $s \in \mathcal{S}$ . Such optimization problems are commonly referred to as linear-fractional programs. For such programs, Charnes and Cooper (1962) show, among other results, that if the feasible set of the program is non-empty and bounded, and if the denominator of the linear-fractional objective is strictly positive for all values in the feasible set, then the linear-fractional program can be transformed to an equivalent linear program—see Boyd and Vandenberghe (2004, Section 4.3.2) for a textbook exposition of this result.

For the linear-fractional programs stated in (S.35), both these conditions are satisfied. Since  $\mathbf{Q}$  is non-empty and bounded, we have that the feasible sets of the programs given by  $\mathbf{Q}$  are indeed non-empty and bounded. Further, since (20) holds for all  $Q \in \mathbf{Q}$ , we also have that the denominator of the objectives are strictly positive for all values in the feasible set. In turn, the result from Charnes and Cooper (1962) can be invoked to transform the linear-fractional programs in (S.35) to equivalent linear programs which are given by those in (22). Specifically, the equivalent linear programs are obtained by introducing the following so-called Charnes-Cooper transformation

$$\tilde{Q}(w) = \gamma \cdot Q(w) \quad \text{where} \quad \gamma = \frac{1}{\sum_{w \in \mathcal{W}_{\text{den}}} Q(w)} , \quad (\text{S.36})$$

which is well-defined given that (20) holds for every  $Q \in \mathbf{Q}$ , and by introducing the additional constraint that  $\gamma \geq 0$ . Then, when the constraints and the objectives stated in terms of  $Q$  for the linear-fractional programs in (S.35) and the relationship between  $Q$  and  $\gamma$  in (S.36) are rewritten in terms of  $\gamma$  and  $\tilde{Q}$ , we obtain the constraints and the objective of the linear programs stated in (22), which concludes the proof.

### S.6.2 Proof of Proposition S.1.1

To begin, since  $C_1 = 1$  by Assumption M4, note that there are two groups of individuals as defined by their potential choice sets in the treatment and control groups:

- (i)  $C_0 = 0$  and  $C_1 = 1$  .

(ii)  $C_0 = 1$  and  $C_1 = 1$  .

The first group complies with their assigned status in the control group and is hence called the complier group. In contrast, the second group does not comply with their assigned status in the control group and is hence, by analogy, called the noncomplier group. For convenience, let  $T$  denote an indicator for whether the individual is a complier or not.

Next, note that we can rewrite the mean observed test scores of those in the treatment group by

$$\begin{aligned} E[Y|Z = 1] &= E[Y_1 \cdot C_1 + Y_0 \cdot (1 - C_1)|Z = 1] \\ &= E[Y_1|Z = 1] \\ &= E[Y_1] , \end{aligned}$$

where the first equality follows from expanding  $Y$  using (S.2) and then expanding  $C$  using (S.3), the second equality follows from Assumption M4, and the third equality follows from Assumption M3. Using the law of total probability, we can then rewrite this quantity in terms of the complier and noncomplier groups, i.e.

$$E[Y|Z = 1] = E[Y_1|T = 1] \cdot \text{Prob}\{T = 1\} + E[Y_1|T = 0] \cdot \text{Prob}\{T = 0\} . \quad (\text{S.37})$$

Similarly, note that we can rewrite the mean observed test scores of those in the control group by

$$\begin{aligned} E[Y|Z = 0] &= E[Y_1 \cdot C_0 + Y_0 \cdot (1 - C_0)|Z = 0] \\ &= E[Y_1 \cdot C_0 + Y_0 \cdot (1 - C_0)] , \end{aligned}$$

where the first equality follows from expanding  $Y$  using (S.2) and then expanding  $C$  using (S.3), and the second equality follows from Assumption M3. Using the law of total probability, we can then again rewrite this quantity in terms of the complier and noncomplier groups, i.e.

$$\begin{aligned} E[Y|Z = 0] &= E[Y_1 \cdot C_0 + Y_0 \cdot (1 - C_0)|T = 1] \cdot \text{Prob}\{T = 1\} + \\ &\quad E[Y_1 \cdot C_0 + Y_0 \cdot (1 - C_0)|T = 0] \cdot \text{Prob}\{T = 0\} \\ &= E[Y_0|T = 1] \cdot \text{Prob}\{T = 1\} + E[Y_1|T = 0] \cdot \text{Prob}\{T = 0\} , \end{aligned} \quad (\text{S.38})$$

where the second equality follows from the fact that  $T = 1$  is by construction equivalent to  $C_0 = 0$  and that  $T = 0$  is equivalent to  $C_0 = 1$ . By taking the difference of the quantities in (S.37) and (S.38), we can then show that the ITT estimand on test scores corresponds to the following

$$\text{ITT}_Y = E[Y|Z = 1] - E[Y|Z = 0] = E[Y_1 - Y_0|T = 1] \cdot \text{Prob}\{T = 1\} . \quad (\text{S.39})$$

In an analogous manner, by replacing the test score  $Y$  with the enrollment decision  $D$ , we can show also that the ITT estimand on enrollment into Head Start corresponds to the following

$$\text{ITT}_D = E[D|Z = 1] - E[D|Z = 0] = E[D_1 - D_0|T = 1] \cdot \text{Prob}\{T = 1\} . \quad (\text{S.40})$$

By recalling that  $1\{T = 1\} \equiv 1\{C_0 = 0, C_1 = 1\}$ , we then obtain the expressions for  $\text{ITT}_D$  and  $\text{ITT}_Y$  stated in the proposition.

To obtain what the IV estimand corresponds to, note that we can rewrite  $\text{ITT}_Y$  in (S.39) using the law of total probability by

$$\begin{aligned} \text{ITT}_Y &= E[Y_1 - Y_0|T = 1, D_1 = 1] \cdot \text{Prob}\{D_1 = 1|T = 1\} \cdot \text{Prob}\{T = 1\} + \\ &\quad E[Y_1 - Y_0|T = 1, D_1 = 0] \cdot \text{Prob}\{D_1 = 0|T = 1\} \cdot \text{Prob}\{T = 1\} \\ &= E[Y_1 - Y_0|T = 1, D_1 = 1] \cdot \text{Prob}\{D_1 = 1|T = 1\} \cdot \text{Prob}\{T = 1\} , \end{aligned} \quad (\text{S.41})$$

where the second equality follows from Assumption M1 and Assumption M2 that together imply that  $D_1 = 0 \implies Y_0 = Y_1$ . Furthermore, since  $D_0 = 0$  by Assumption M1, it follows that  $\text{ITT}_D$  in (S.40) can be rewritten as

$$\text{ITT}_D = \text{Prob}\{D_1 = 1|T = 1\} \cdot \text{Prob}\{T = 1\} . \quad (\text{S.42})$$

In turn, by taking the ratio of  $\text{ITT}_Y$  and  $\text{ITT}_D$  as stated in (S.41) and (S.42), we can then show that the IV estimand corresponds to the following

$$\text{IV} = E[Y_1 - Y_0|T = 1, D_1 = 1] .$$

Again, by recalling that  $1\{T = 1\} \equiv 1\{C_0 = 0, C_1 = 1\}$ , we then obtain the expression for IV stated in the proposition, which concludes the proof.

### S.6.3 Rewriting Assumptions in Section 3.4 in terms of (17)

Similar to Assumption HSIS, the identifying content that the assumptions in Section 3.4 provide in terms of the parameters of interest can be characterized using Proposition 3.1 from Section 3.3. As noted, this is due to the fact that each of these assumptions can be re-written as restrictions on  $Q$  in the form of (17). In particular, similar to Assumption HSIS(ii), it is straightforward to see that Assumption UA can be re-written in terms of  $Q$  as

$$\sum_{w \in \mathcal{W}_{\text{UA}}} Q(w) = 0 , \quad (\text{S.43})$$

where  $\mathcal{W}_{\text{UA}} = \{w \in \mathcal{W} : a \in c(0), a \notin c(1) \text{ or } a \notin c(0), a \in c(1)\}$ , and also that Assumption MTR can be re-written in terms of  $Q$  as

$$\sum_{w \in \mathcal{W}_{\text{MTR}}} Q(w) = 0 , \quad (\text{S.44})$$

where  $\mathcal{W}_{\text{MTR}} = \{w \in \mathcal{W} : y(n) > y(h) \text{ or } y(n) > y(a)\}$ . In order to see the restrictions imposed by Assumption Roy, note first this assumption can be equivalently stated as

$$d(U, \{d, d'\}) = d \implies Y(d') \leq Y(d)$$

for each  $d, d' \in \mathcal{D}$ . Then, it follows that Assumption **Roy** can also be re-written in terms of  $Q$  as

$$\sum_{w \in \mathcal{W}_{\text{Roy}, \{d, d'\}}} Q(w) = 0 , \quad (\text{S.45})$$

for all  $d, d' \in \mathcal{D}$ , where  $\mathcal{W}_{\text{Roy}, \{d, d'\}} = \{w \in \mathcal{W} : y(d') > y(d), u \in \mathcal{U}_{\{d, d'\}}\}$  and  $\mathcal{U}_{\{d, d'\}} = \{u \in \mathcal{U} : d(u, \{d, d'\}) = d\}$ .

## References

- ANGELUCCI, M., KARLAN, D. and ZINMAN, J. (2015). Microcredit impacts: Evidence from a randomized microcredit program placement experiment by compartamos banco. *American Economic Journal: Applied Economics*, **7** 151–82.
- BOYD, S. and VANDENBERGHE, L. (2004). *Convex optimization*. Cambridge university press.
- CHARNES, A. and COOPER, W. W. (1962). Programming with linear fractional functionals. *Naval Research Logistics (NRL)*, **9** 181–186.
- DEB, R., KITAMURA, Y., QUAH, J. K.-H. and STOYE, J. (2018). Revealed price preference: Theory and empirical analysis. *arXiv preprint arXiv:1801.02702*.
- FELLER, A., GRINDAL, T., MIRATRIX, L. and PAGE, L. C. (2016). Compared to what? variation in the impacts of early childhood education by alternative care type. *The Annals of Applied Statistics*, **10** 1245–1285.
- FINKELSTEIN, A., TAUBMAN, S., WRIGHT, B., BERNSTEIN, M., GRUBER, J., NEWHOUSE, J. P., ALLEN, H., BAICKER, K. and GROUP, O. H. S. (2012). The oregon health insurance experiment: evidence from the first year. *The Quarterly journal of economics*, **127** 1057–1106.
- HOROWITZ, J. L. and MANSKI, C. F. (1995). Identification and robustness with contaminated and corrupted data. *Econometrica: Journal of the Econometric Society* 281–302.
- IMBENS, G. W. and ANGRIST, J. D. (1994). Identification and estimation of local average treatment effects. *Econometrica*, **62** 467–475.
- IMBENS, G. W. and RUBIN, D. B. (2015). *Causal Inference for Statistics, Social, and Biomedical Sciences: An Introduction*. Cambridge University Press.
- KITAMURA, Y. and STOYE, J. (2018). Nonparametric analysis of random utility models. *Econometrica*, **86** 1883–1909.
- KLINE, P. and SANTOS, A. (2013). Sensitivity to missing data assumptions: Theory and an evaluation of the us wage structure. *Quantitative Economics*, **4** 231–267.
- KLINE, P. and WALTERS, C. R. (2016). Evaluating public programs with close substitutes: The case of head start. *The Quarterly Journal of Economics*, **131** 1795–1848.
- MASTEN, M. A. and POIRIER, A. (2017). Inference on breakdown frontiers. *arXiv preprint arXiv:1705.04765*.
- MOGSTAD, M. and TORGOVITSKY, A. (2018). Identification and extrapolation of causal effects with instrumental variables. *Annual Review of Economics*.
